# Supplementary material for: CLIP-GEN: Language-Free Training of a Text-to-Image Generator with CLIP
Source: arXiv:2203.00386 source file (2022-03-01)
Supplement: Supplementary file 1 [file supp.tex]

% CVPR 2022 Paper Template
% based on the CVPR template provided by Ming-Ming Cheng (https://github.com/MCG-NKU/CVPR_Template)
% modified and extended by Stefan Roth (stefan.roth@NOSPAMtu-darmstadt.de)

\documentclass[10pt,twocolumn,letterpaper]{article}

\usepackage[camera]{cvpr}  

% Include other packages here, before hyperref.
\usepackage{graphicx}
\usepackage{amsmath}
\usepackage{amssymb}
\usepackage{booktabs}
\usepackage{color}
\usepackage{subfiles}
\usepackage{mmstyles}

% It is strongly recommended to use hyperref, especially for the review version.
% hyperref with option pagebackref eases the reviewers' job.
% Please disable hyperref *only* if you encounter grave issues, e.g. with the
% file validation for the camera-ready version.
%
% If you comment hyperref and then uncomment it, you should delete
% ReviewTempalte.aux before re-running LaTeX.
% (Or just hit 'q' on the first LaTeX run, let it finish, and you
%  should be clear).
\usepackage[pagebackref,breaklinks,colorlinks]{hyperref}

% Support for easy cross-referencing
\usepackage[capitalize]{cleveref}
\crefname{section}{Sec.}{Secs.}
\Crefname{section}{Section}{Sections}
\Crefname{table}{Table}{Tables}
\crefname{table}{Tab.}{Tabs.}

%%%%%%%%% PAPER ID  - PLEASE UPDATE
 % *** Enter the CVPR Paper ID here

\begin{document}

%%%%%%%%% TITLE - PLEASE UPDATE

\twocolumn[{%
\renewcommand\twocolumn[1][]{#1}%
\begin{center}
      % smaller title font only for rebuttal
     {\Large \bf CLIP-GEN: Language-Free Training of a Text-to-Image Generator with CLIP \\ \rule{2cm}{0.7pt} \\Supplementary Material \par}
      % additional two empty lines at the end of the title
      {
      \large
      \lineskip .5em
      \par
      }
      % additional small space at the end of the author name
      \vskip .5em
      % additional empty line at the end of the title block
      \vspace*{12pt}
  \end{center}
}]

%\maketitle

In this supplementary material, we provide additional implementation details, as well as some additional visual results.

In~\cref{sec:implementation}, we present the architecture and hyperparameters we used during training. In ~\cref{sec:res}, we show additional generated images with different sample strategies, and some generated illustrations for famous lines of poetry.

\iffalse
\section{Implementation Details}
\label{sec:implementation}

\noindent\textbf{VQ-GAN Training} In the pre-training stage, we train two VQ-GAN models on ImageNet and COCO dataset respectively. Both models have the same architecture and hyperparameters. Specifically, we set the codebook size $|\cZ|=16384$, embedding size $dim_z=256$, compression factor $f=16$ and sequence length $|s|=16\times 16=256$.

Following the implementation of the original VQ-GAN, we use a 3-layer PatchGAN discriminator with perception loss.  The model is trained for 100 epochs with a batch size of 16. The discriminator is not trained for the first 25,000 steps. The models are trained via Adam optimizer with the initial learning rate of 4.5e-6. During training, input images are resized and random cropped to $256\times 256$ while the model leanrs to reconstruct the image of the same size.

\noindent\textbf{Self-supervised Training of the Auto-regressive Transformer} In the second stage, we only train the auto-regressive transformer, while the weights of VQ-GAN and CLIP are fixed. We choose the GPT-2 architecture in our implementation. We use the GPT-2-Medium model for the COCO dataset and the GPT-2-XL model for the ImageNet dataset.
\fi

\subfile{supp_sections/implementation.tex}
\subfile{supp_sections/results.tex}

\end{document}
